# Supplementary material for: Sound reconstruction from human brain activity via a generative model with brain-like auditory features
Source: arXiv:2306.11629 source file (2023-06-20)
Supplement: Supplementary file 1 [file 03_Article_SupplementaryVideos.tex]

%  CONFIGURE NEW SINGLE-PAGE FORMAT 

\onecolumn % go back to one column
\fancyhead{} % make sure we get no headers

\lfoot[\bSupInf]{\dAuthor}
\rfoot[\dAuthor]{\cSupInf}
\newpage

\captionsetup*{format=largeformat} % make figure legend slightly larger than in the paper
\setcounter{figure}{0} % reset figure counter for Supplementary Video Figures
\makeatletter 
\renewcommand{\thefigure}{SV\@arabic\c@figure} % make Figure legend start with Figure S
\makeatother

%  MAIN TEXT 
\newpage
\section*{Supplementary Videos}

\begin{SCfigure*}[50][!ht]
\includegraphics[width=0.5\linewidth]{Figures/temp.png}
\caption{\textbf{This is a video of a lysosome.}\\
A typical caption would go here. We use a thumbnail version of the video file as the figure.\\
Time, seconds. Scale bar, \SI{10}{\micro\meter}.}
\label{videosupp:lysosome}
\end{SCfigure*}
